# Supplementary material for: Cross-Domain Latent Modulation for Variational Transfer Learning
Source: arXiv:2012.11727 source file (2020-12-21)
Supplement: Supplementary file 1 [file appendices.tex]

%\appendices

% \section{Supplementary}
\subsection{Reparameterization for Variational Cross-Domain Generation} \label{supp:repara-cross-domain}

In our model, the reparameterization can be written as follows:

\begin{equation}
  \begin{gathered}
    \bm{\ddot{z}}_{st} = \mathcal{G}((\bm \mu_s, \bm \sigma_s), \bm h_t) = \bm \mu_s + \bm \sigma_s \odot (\gamma_1\bm h_t + \gamma_2\bm \epsilon) \\
    \bm {\ddot{z}}_{ts} = \mathcal{G}((\bm \mu_t, \bm \sigma_t), \bm h_s) = \bm \mu_t + \bm \sigma_t \odot (\gamma_1\bm h_s + \gamma_2\bm \epsilon),
    \end{gathered}
    \label{eq:z_addition_appe}
\end{equation}
%where $i$ means the $i$th element. 
In general, consider $\bm h_s \sim p(\mathcal{H}_s) = \mathcal{N}(\bm \mu_{\bm h_s}, \bm \sigma_{\bm h_s})$, and $\bm h_t \sim p(\mathcal{H}_t) = \mathcal{N}(\bm \mu_{\bm h_t}, \bm \sigma_{\bm h_t})$. Adding the standard Gaussian distribution, $\epsilon \sim p(\epsilon) = \mathcal{N}(0, \mathbf{I})$, from Eq.(\ref{eq:z_addition_appe}) we have  $\bm{\ddot{z}}_{st} \sim \mathcal{N}(\bm{\ddot{z}}_{st}; \bm \mu_{st}, \bm \sigma_{st}^2\mathbf{I})$. The $i$-th element of its mean vector can be obtained as
\begin{equation}
\begin{split}
    \mu_{st}^i &= \mathbb{E}\{\mu^i_s + \sigma_s^i(\gamma_1 h_t^i + \gamma_2 \epsilon^i)\}\\
    & = \mu_s^i + \sigma_s^i\gamma_1 E\{h_t\} + \gamma_2 E\{\epsilon^i\} \\
    &= \mu_s^i + \gamma_1 \sigma_s^i \mu_{h_t}^i.
\end{split}
\end{equation}

Ignoring the bias term $\mu_s$, we have the $i$-th element of the variance vector:

\begin{equation}
    \begin{split}
        \mathbf{Var}(\ddot{z}_{st}^i) &= \mathbf{Var}[\sigma_s^i (\gamma_1 h_t^i + \gamma_2 \epsilon^i)]\\
        &=\mathbb{E}\{(\sigma_s^i(\gamma_1 h_t^i + \gamma_2\epsilon^i) - \gamma_1\sigma_s^i\mu_{h_t}^i)^2\} \\
        &= (\sigma_s^i)^2 \mathbb{E}\{[ (\gamma_1 h_t^i + \gamma_2\epsilon^i) - \gamma_1\mu_{h_t}^i]^2\} \\
        &= (\sigma_s^i)^2 \left( \mathbb{E}\{[ (\gamma_1 h_t^i + \gamma_2\epsilon^i)]^2\} - (\gamma_1 \mu_{h_t}^i)^2 \right) \\
        &= (\sigma_s^i)^2 [\gamma_1^2(\sigma_{h_t}^i)^2 + \gamma_2^2].
    \end{split}
\end{equation}
Therefore, the $i$-th element of the standard deviation vector $\bm\sigma_{st}$ is
\begin{equation}
    \sigma_{st}^i = \sigma_s^i \sqrt{\gamma_1^2(\sigma_{h_t}^i)^2 + \gamma_2^2}. 
\end{equation}

There is similar formulation for $\mu_{ts}^i$ and $\sigma_{ts}^i$, as follows:
\begin{equation}
\begin{gathered}
\mu_{ts}^i = \mu_t^i + \gamma_1 \sigma_t^i \mu_{h_s}^i \\
\sigma_{ts}^i = \sigma_t^i \sqrt{\gamma_1^2(\sigma_{h_s}^i)^2 + \gamma_2^2}
\end{gathered}
\end{equation}

\subsection{Experiments Settings}
\label{supp:experiments_setting}
See Tables 5 -- 6.

\begin{table*}[]
    \centering
    \caption{Experiments Setting for Unsupervised Domain Adaptation}
    \resizebox{1.0\textwidth}{!}{
        \begin{tabular}{|c|c|c|c|c|c|c|c|c|c|c|}
            \hline
            \multirow{2}{*}{Experiments} & \multirow{2}{*}{enc\_style}  & \multirow{2}{*}{Encoder} & \multirow{2}{*}{Decoder} & \multirow{2}{*}{Discriminator} & \multicolumn{2}{|c|}{Encoder Updating} & \multicolumn{2}{|c|}{Decoder Updating} & \multicolumn{2}{|c|}{cls for pixel UDA}   \\
            \cline{6-11}
            &  &    &   &   & LR ($\eta_1$) & optimizer & LR ($\eta_2$) & optimizer &  LR & optimizer  \\
            \hline
            MNIST-MNISTM & fc (128*8)  & \makecell{f32k5s1-\\bn-\\f64k5s2-\\bn-\\f64k5s1-\\bn-\\f128k8s1-\\bn-\\f256k1s2-\\bn-\\f256k1s1}  & \makecell{f128k4s2-\\bn-\\f128k4s1-\\bn-\\f128k4s1-\\bn-\\f64k4s1-\\bn-\\f32k4s2-\\bn-\\f3k1s1}  & fc100-fc2  & \makecell{0.01\\annealing} & \makecell{Momentum-\\SGD (0.6)} & 0.0002  & \makecell{Adam \\($\beta_1$=0.5, \\ $\beta_2$=0.999)} & 0.001  & \makecell{Adam\\($\beta_1$=0.5,\\ $\beta_2$=0.999)}  \\
            \hline
            MNISTM-MNIST & fc (128*8) & - & - & - &\makecell{0.01\\annealing} & \makecell{Momentum-\\SGD (0.8)} & 0.2 & \makecell{Adam \\($\beta_1$=0.5, \\ $\beta_2$=0.999)} & 0.001 & \makecell{Adam\\($\beta_1$=0.5, \\ $\beta_2$=0.999)}  \\
            \hline
            MNIST-USPS & fc (128*8) & - & - & - &\makecell{0.01\\annealing} & \makecell{Momentum-\\SGD (0.8)} & 0.0002 & \makecell{Adam \\($\beta_1$=0.5, \\ $\beta_2$=0.999)} & 0.001 & \makecell{Adam\\($\beta_1$=0.5, \\ $\beta_2$=0.999)}  \\
            \hline
            USPS-MNIST & fc (128*8) & - & - & -  &\makecell{0.01\\annealing} & \makecell{Momentum-\\SGD (0.9)} & 0.001 & \makecell{Adam \\($\beta_1$=0.5, \\ $\beta_2$=0.999)} & 0.0008 & \makecell{Adam\\($\beta_1$=0.5, \\ $\beta_2$=0.999)}  \\
            \hline
            FASHION-FASHIONM & fc (128*8) & - & - & - &\makecell{0.01\\annealing} & \makecell{Momentum-\\SGD (0.8)} & 0.001 & \makecell{Adam \\($\beta_1$=0.5, \\ $\beta_2$=0.999)} & 0.001 & \makecell{Adam\\($\beta_1$=0.5, \\ $\beta_2$=0.999)}  \\
            \hline
            FASHIONM-FAHSION & fc (128*8) & -  & - & - &\makecell{0.01\\annealing} & \makecell{Momentum-\\SGD (0.9)} & 0.01 & \makecell{Adam \\($\beta_1$=0.5, \\ $\beta_2$=0.999)} & 0.001 & \makecell{Adam\\($\beta_1$=0.5, \\ $\beta_2$=0.999)}  \\
            \hline
            Linemod-linemod3D & fc (128*8) & - & - & - &\makecell{0.01\\annealing} & \makecell{Momentum-\\SGD (0.6)} & 2e-5 & \makecell{Adam \\($\beta_1$=0.5, \\ $\beta_2$=0.999)} & 0.0001 & \makecell{Adam\\($\beta_1$=0.5, \\ $\beta_2$=0.999)} \\
            \hline
    \end{tabular}}
\end{table*} 

\begin{table*}[]
    \centering
    \caption{Experiments Setting for Unsupervised Image Translation}
    \resizebox{1.0\textwidth}{!}{
        \begin{tabular}{|c|c|c|c|c|c|c|c|c|}
            \hline
            \multirow{2}{*}{Experiments} & \multirow{2}{*}{enc\_style}  & \multirow{2}{*}{Encoder} & \multirow{2}{*}{Decoder} & \multirow{2}{*}{Discriminator} & \multicolumn{2}{|c|}{Encoder Updating} & \multicolumn{2}{|c|}{Decoder Updating} \\
            \cline{6-9}
            &  &    &   &   & LR ($\eta_1$) & optimizer & LR ($\eta_2$) & optimizer \\
            \hline
            Shoes-edge & fc (128*8)  & \makecell{f32k5s1-\\bn-\\f64k5s2-\\bn-\\f64k5s1-\\bn-\\f128k8s1-\\bn-\\f256k1s2-\\bn-\\f256k1s1} & \makecell{f128k4s2-\\bn-\\f128k4s1-\\bn-\\f128k4s1-\\bn-\\f64k4s1-\\bn-\\f32k4s2-\\bn-\\f3k1s1} & fc100-fc2  & \makecell{0.01\\annealing} & \makecell{Momentum-\\SGD (0.4)} & 0.002  & \makecell{Adam \\($\beta_1$=0.5, \\ $\beta_2$=0.999)}  \\
            \hline
            edge-Shoes & fc (128*8) & - & - & -  &\makecell{0.01\\annealing} & \makecell{Momentum-\\SGD (0.6)} & 0.02 & \makecell{Adam \\($\beta_1$=0.5, \\ $\beta_2$=0.999)} \\
            \hline
            CelebA-Sketched CelebA & fc (128*8) & - & - & -  &\makecell{0.01\\annealing} & \makecell{Momentum-\\SGD (0.6)} & 0.2 & \makecell{Adam \\($\beta_1$=0.5, \\ $\beta_2$=0.999)}  \\
            \hline
            Sketched CelebA-CelebA & fc (128*8) & - & - & -   &\makecell{0.01\\annealing} & \makecell{Momentum-\\SGD (0.6)} & 0.2 & \makecell{Adam \\($\beta_1$=0.5, \\ $\beta_2$=0.999)}  \\
            \hline
    \end{tabular}}
\end{table*}

\subsection{More Generation Images}
\label{supp:more_generations}
See Figures 8 -- 18.

\begin{figure*}[thbp]
   \centering
   \includegraphics[width=1.0\textwidth]{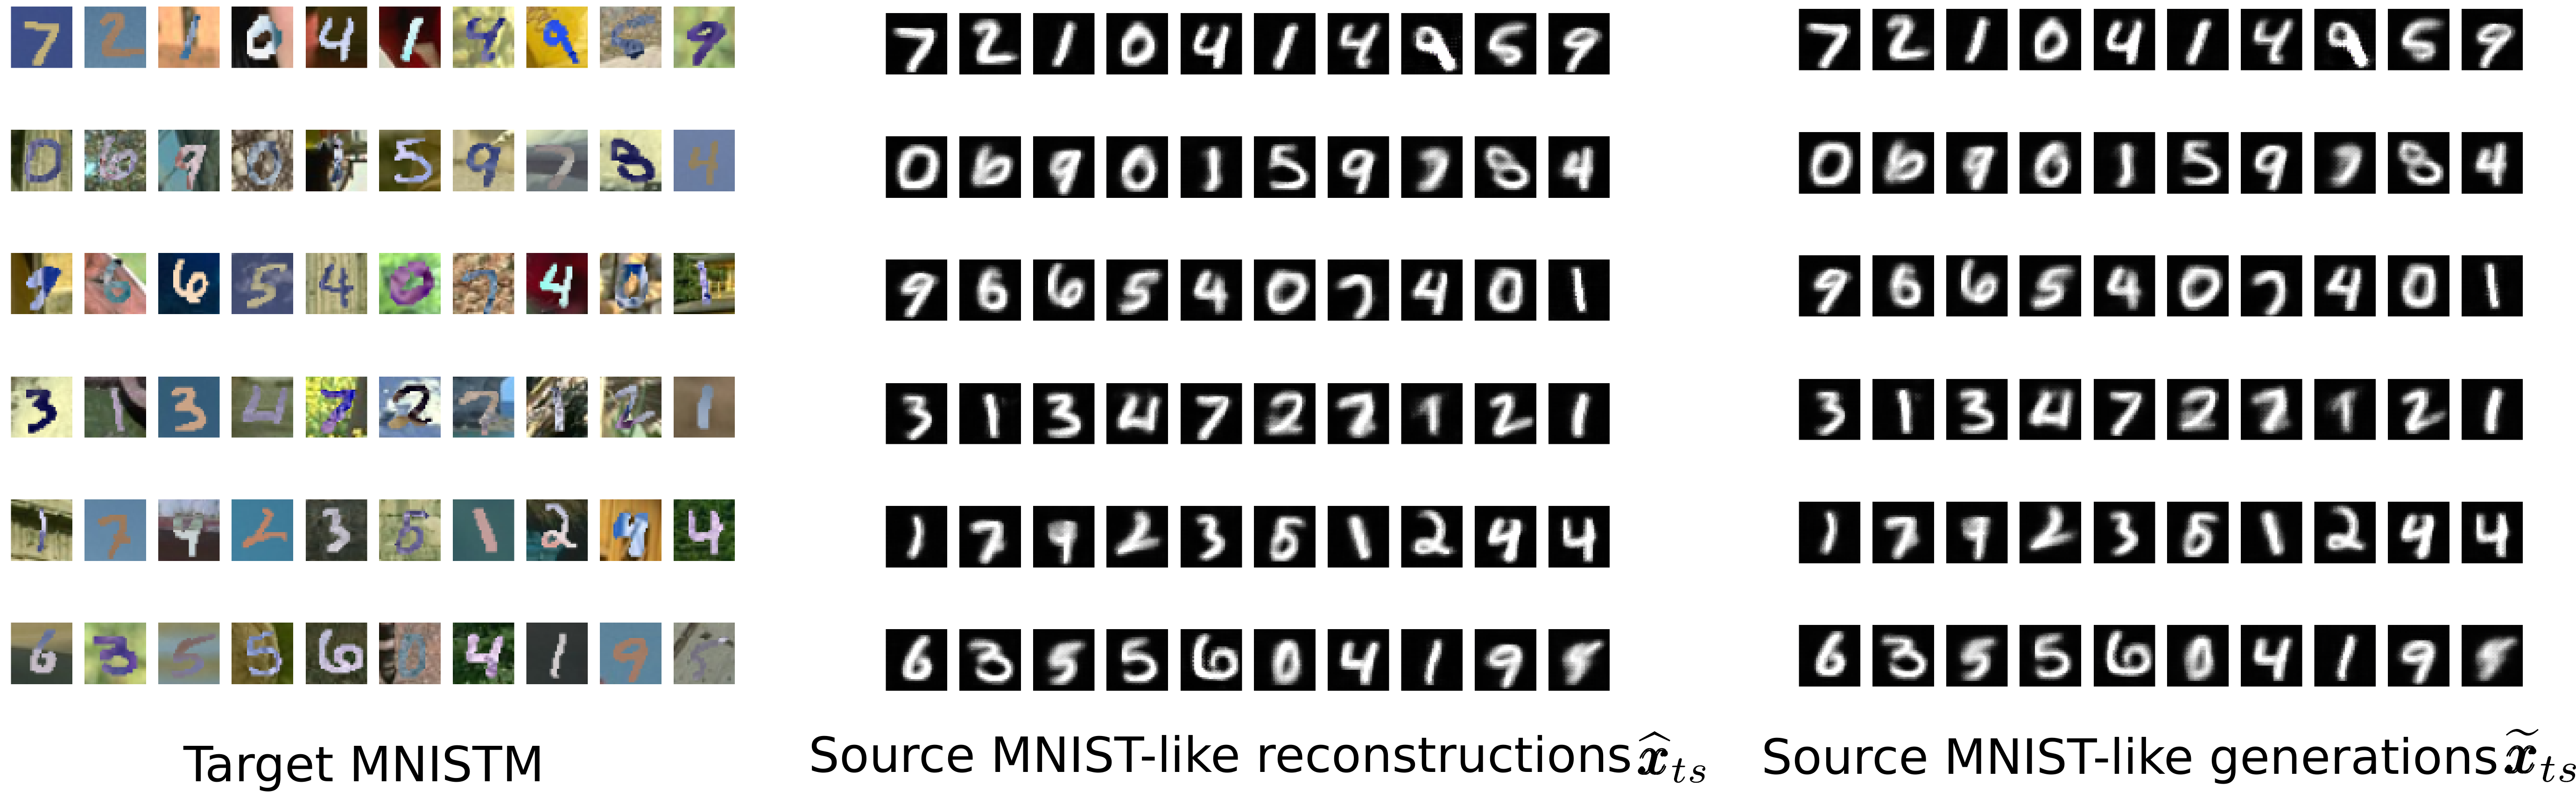}
   \caption{More Generations in task MNIST(source)-MNISTM(target)}
   \label{fig:mnist_mnistm_more}
\end{figure*}

\begin{figure*}[thbp]
   \centering
   \includegraphics[width=1.0\textwidth]{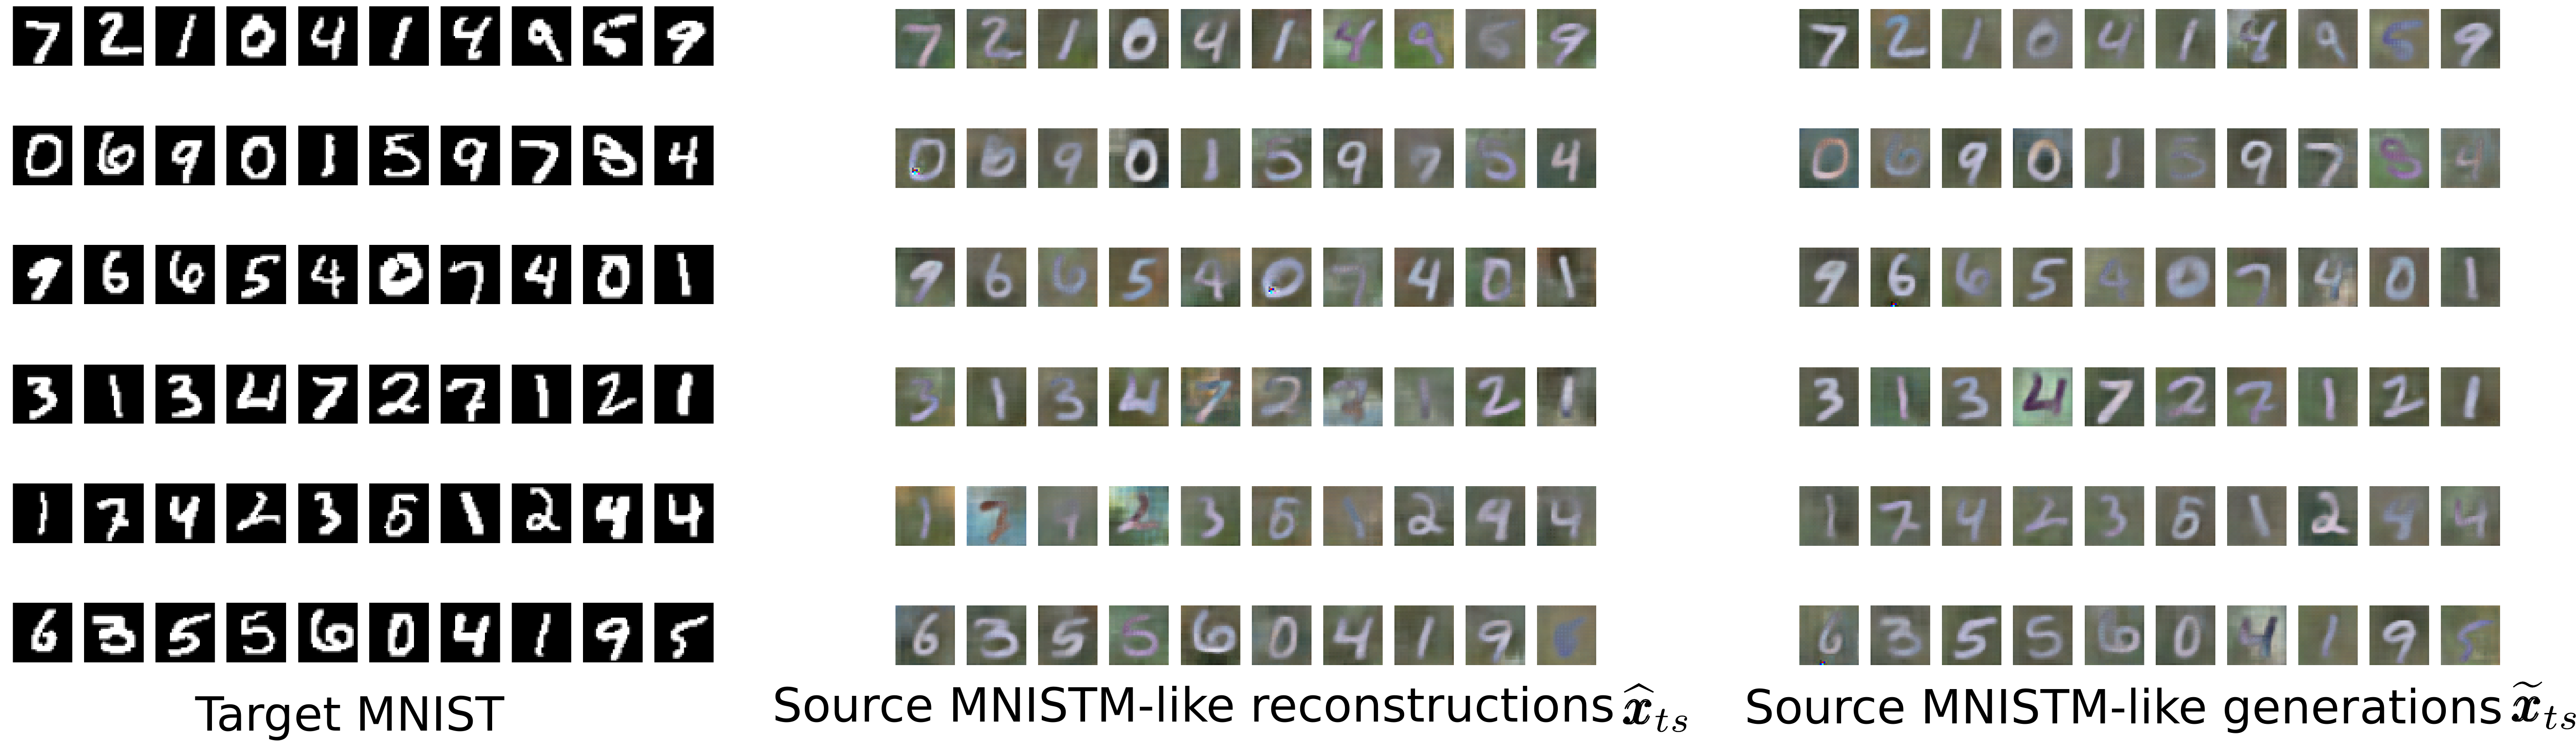}
   \caption{More Generations in task MNISTM(source) -- MNIST(target)}
   \label{fig:mnistm_mnist_more}
\end{figure*}

\begin{figure*}[thbp]
   \centering
   \includegraphics[width=1.0\textwidth]{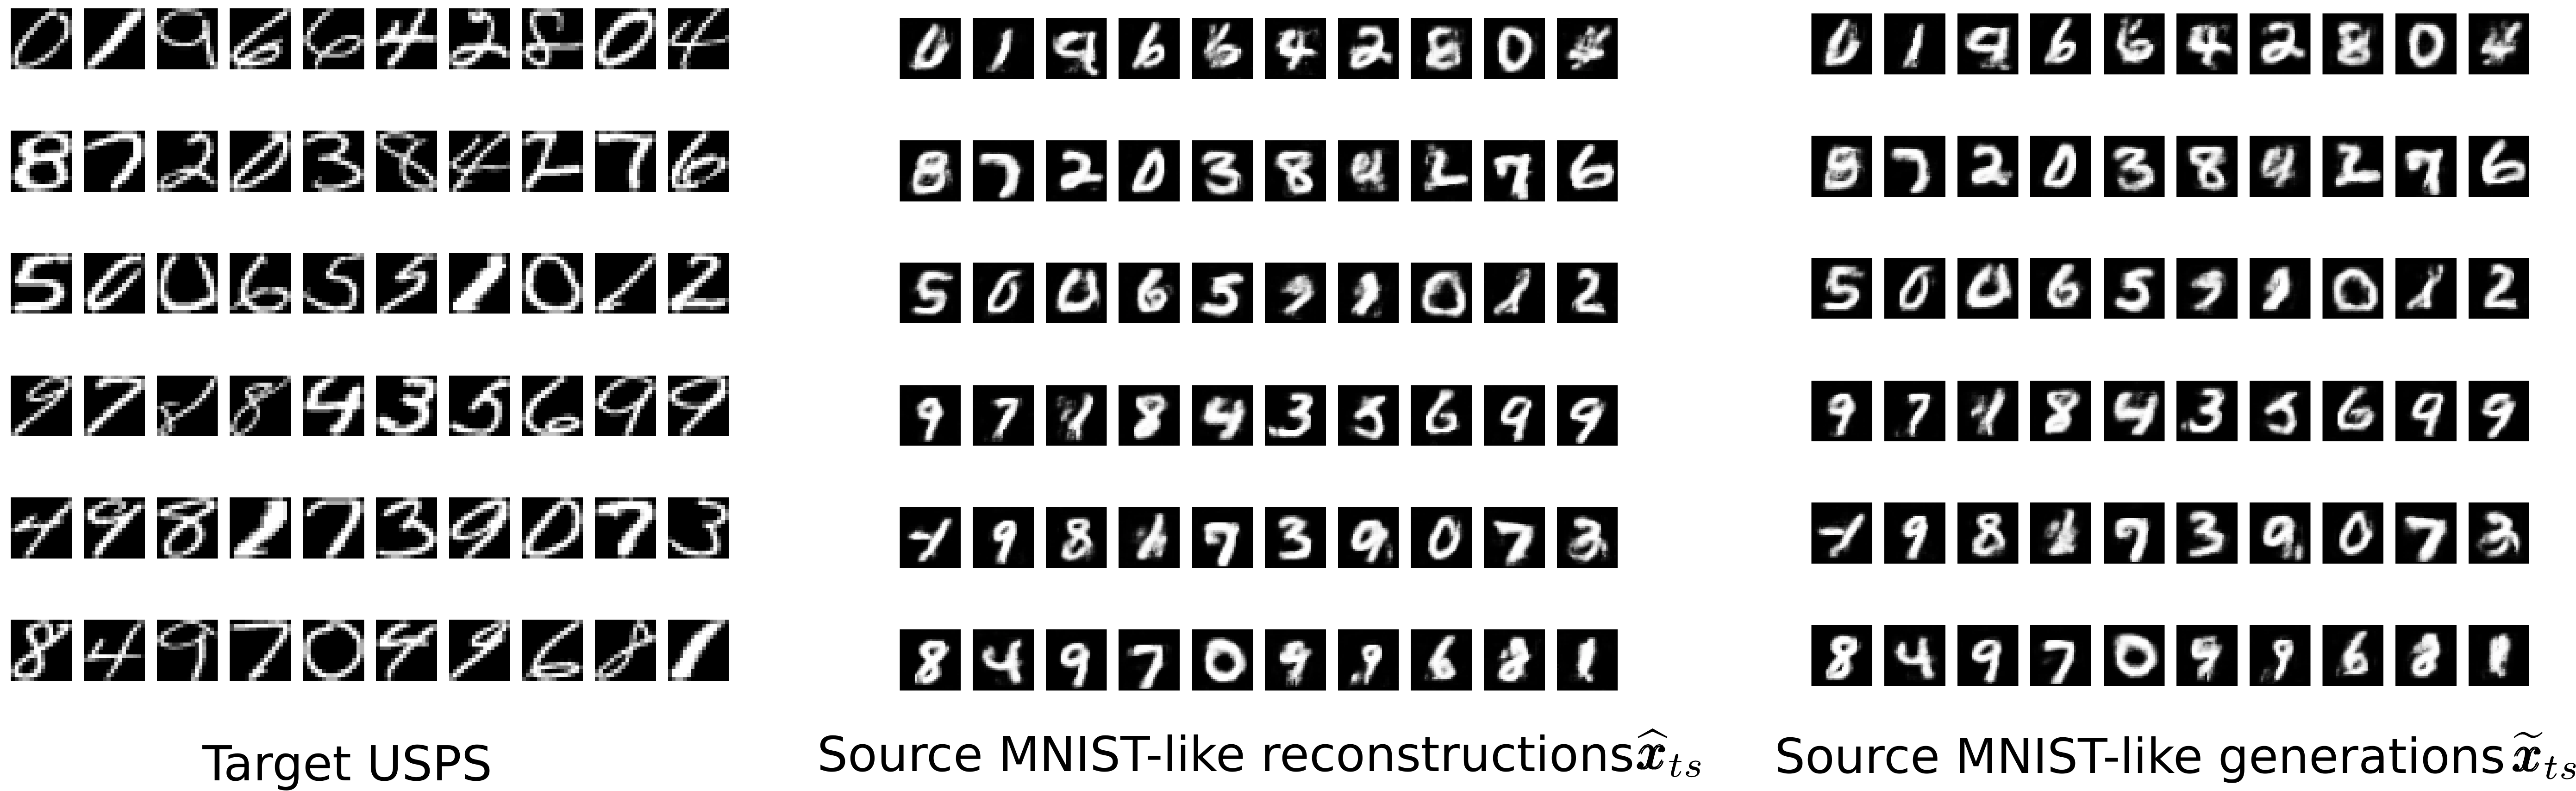}
   \caption{More Generations in task MNIST(source) -- USPS(target)}
   \label{fig:mnist_usps_more}
\end{figure*}

\begin{figure*}[thbp]
   \centering
   \includegraphics[width=1.0\textwidth]{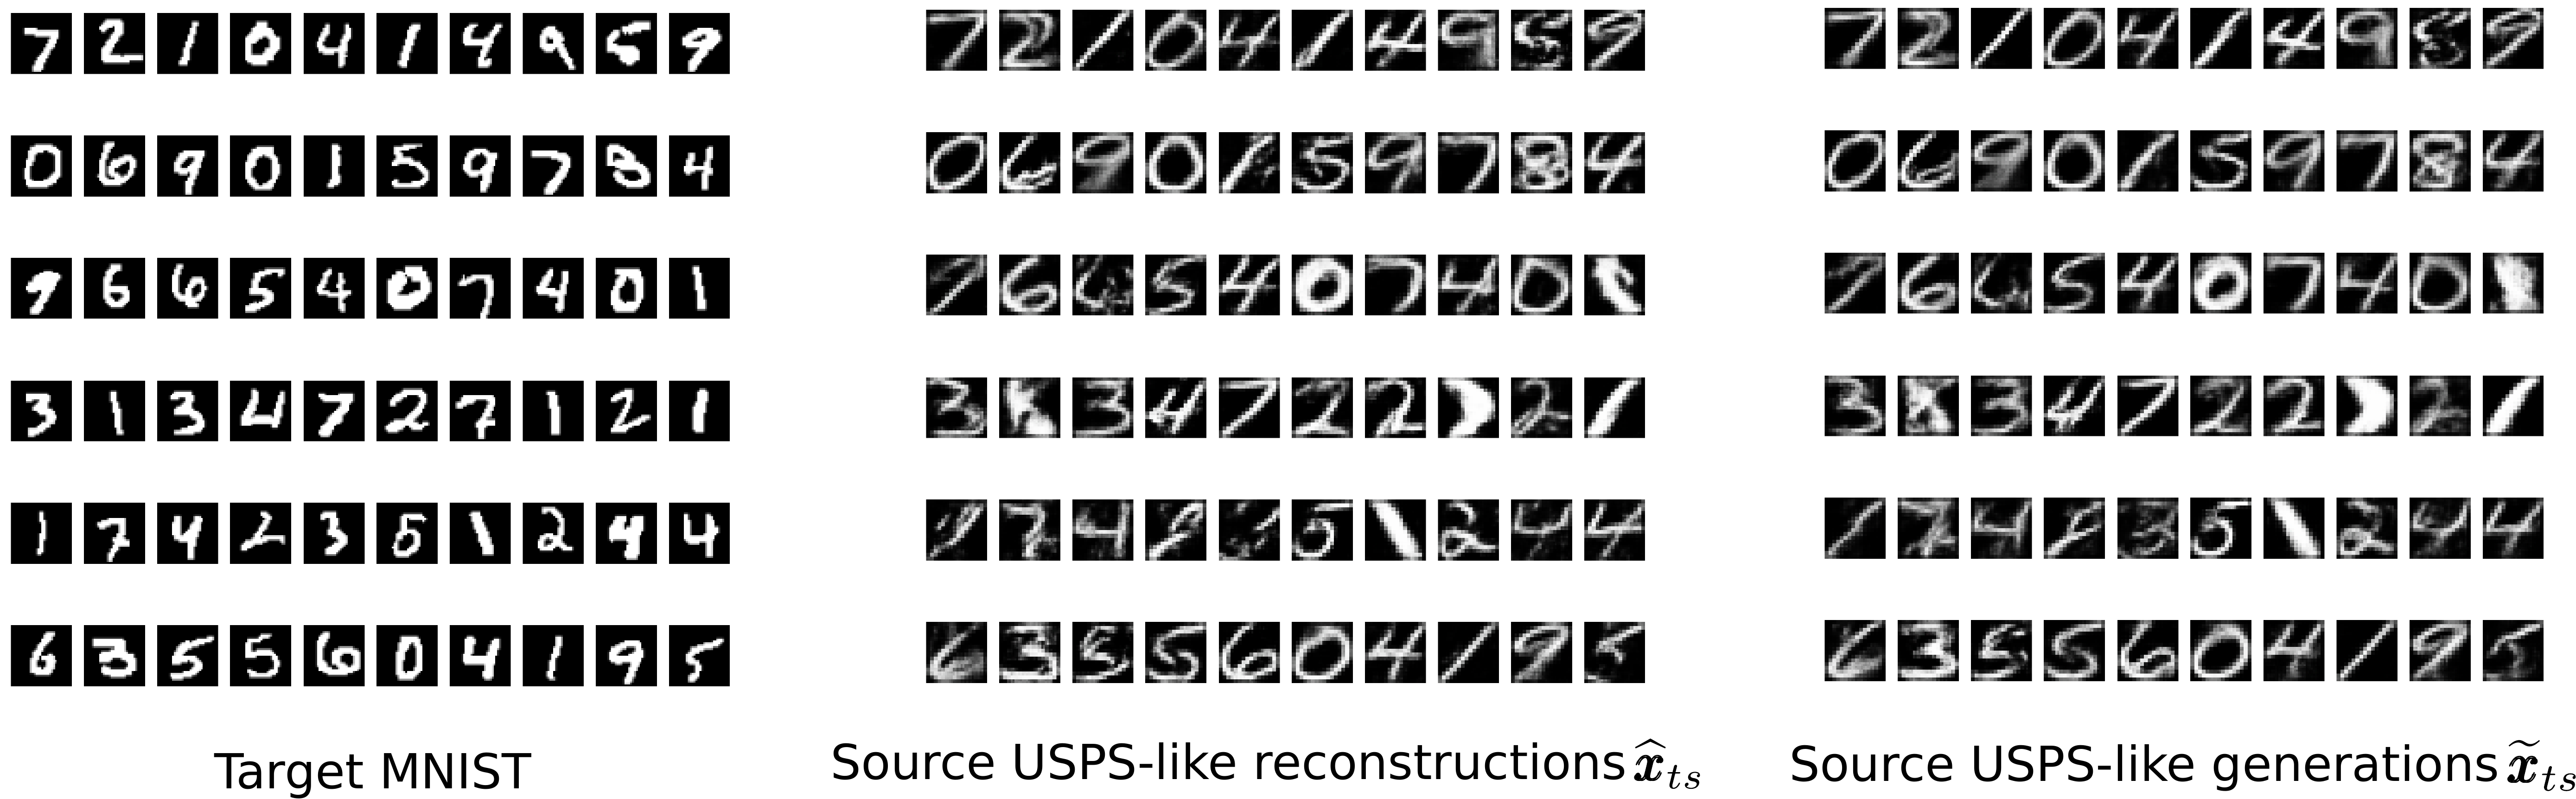}
   \caption{More Generations in task USPS(source) -- MNIST(target)}
   \label{fig:usps_mnist_more}
\end{figure*}

\begin{figure*}[thbp]
   \centering
   \includegraphics[width=1.0\textwidth]{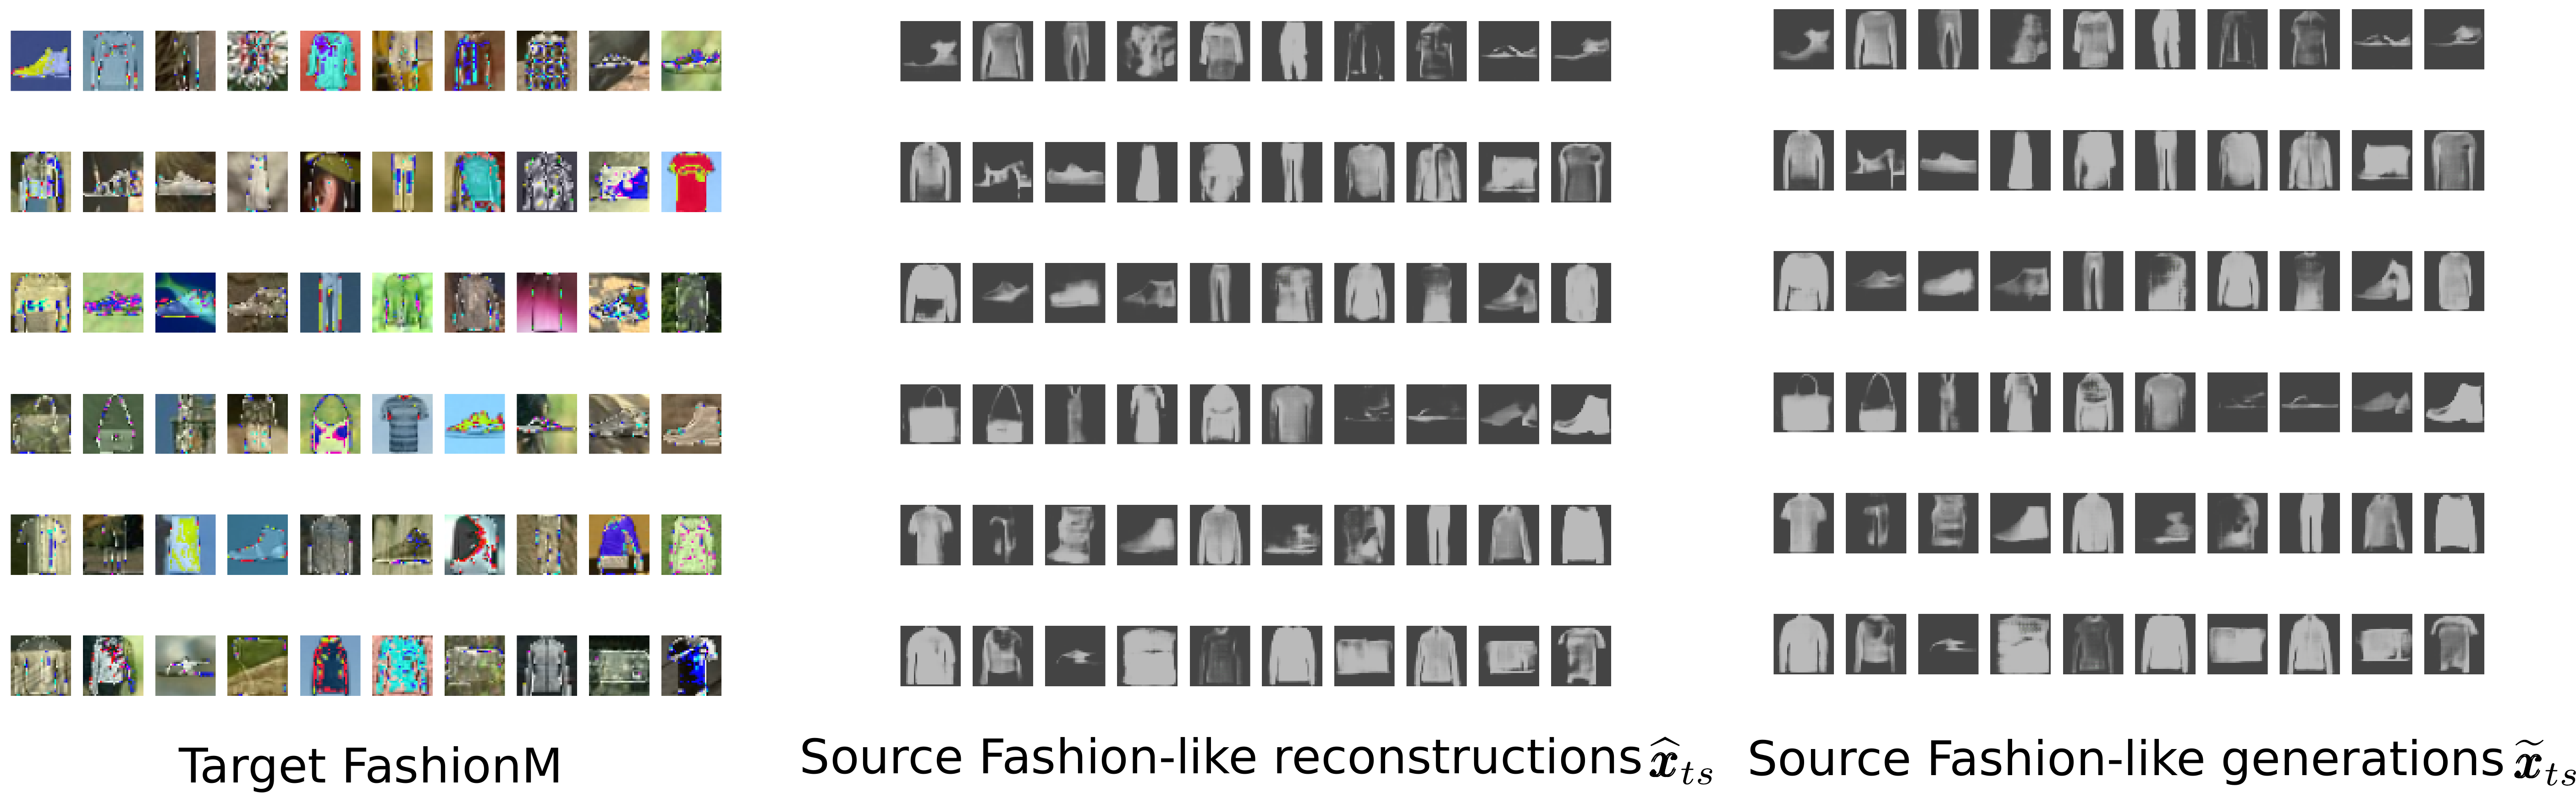}
   \caption{More Generations in task Fashion(source) -- FashionM(target)}
   \label{fig:fashion_fashionm_more}
\end{figure*}

\begin{figure*}[thbp]
   \centering
   \includegraphics[width=1.0\textwidth]{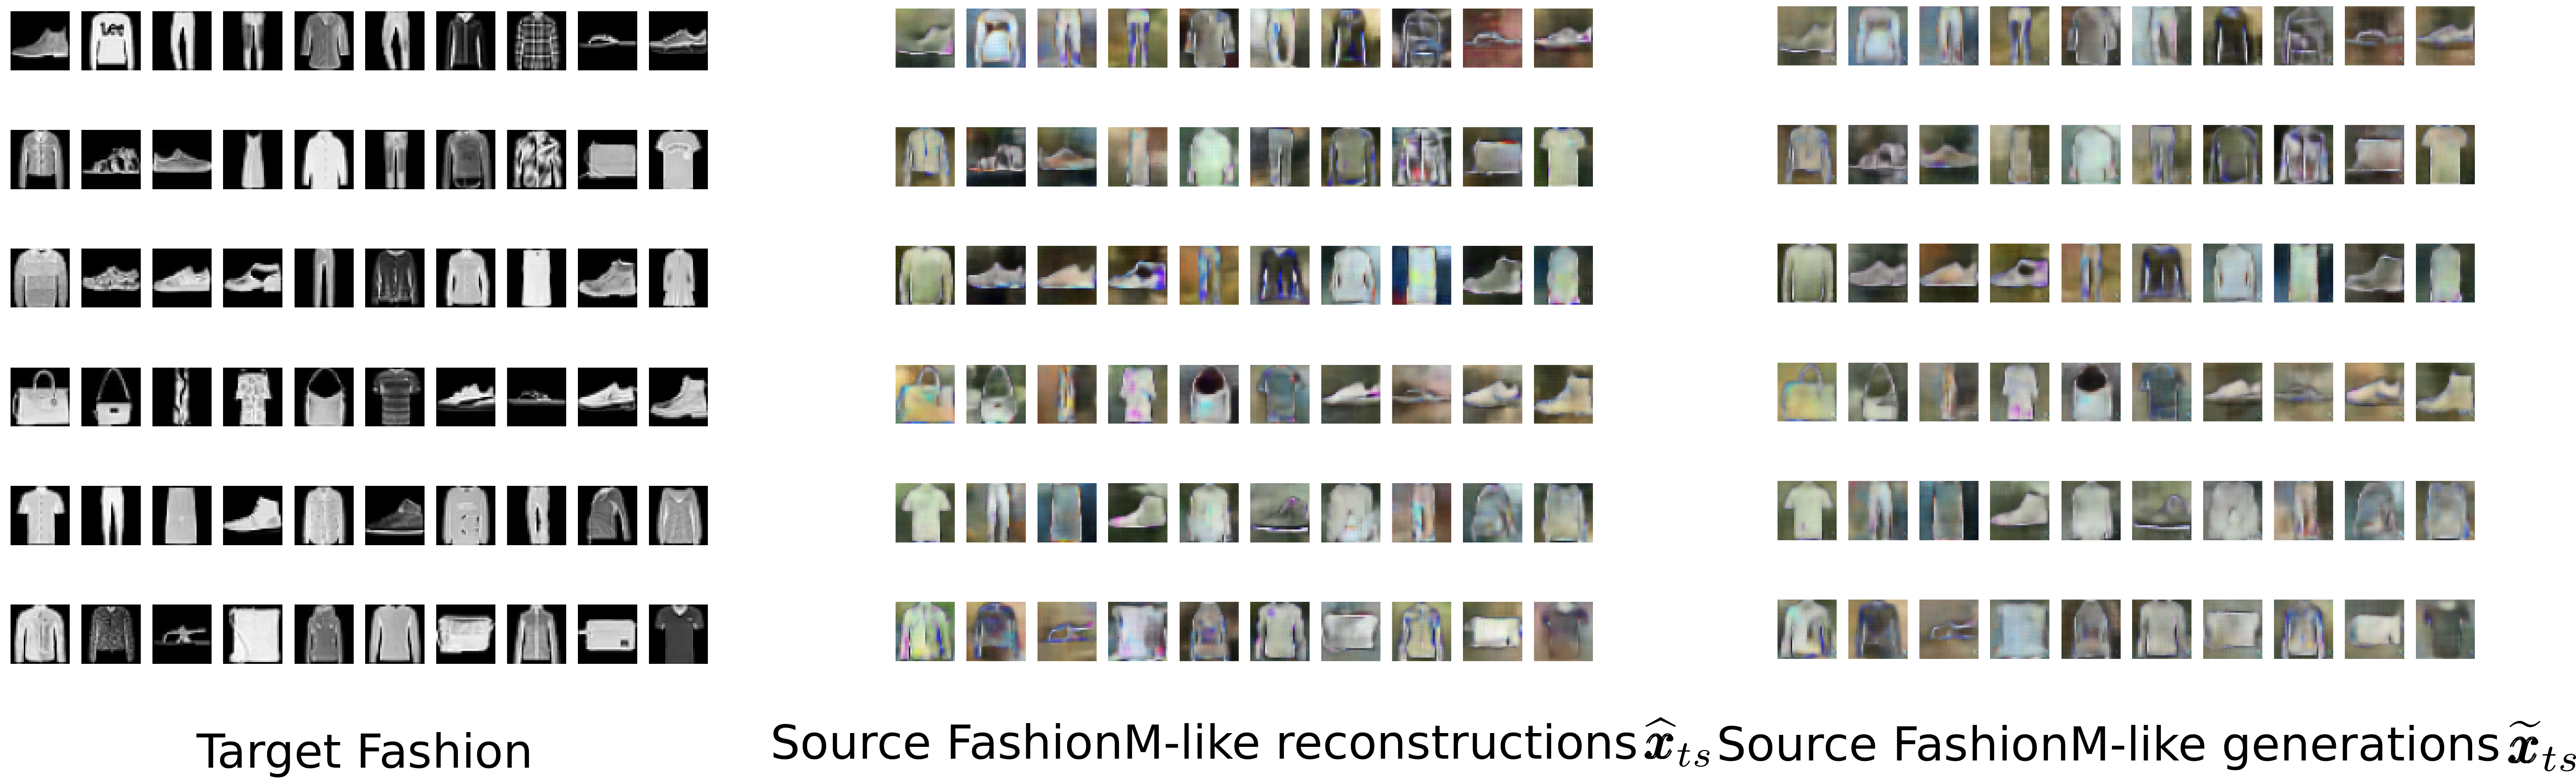}
   \caption{More Generations in task FashionM(source) -- Fashion(target)}
   \label{fig:fashionm_fashion_more}
\end{figure*}

\begin{figure*}[thpb]
   \centering
   \includegraphics[width=1.0\textwidth]{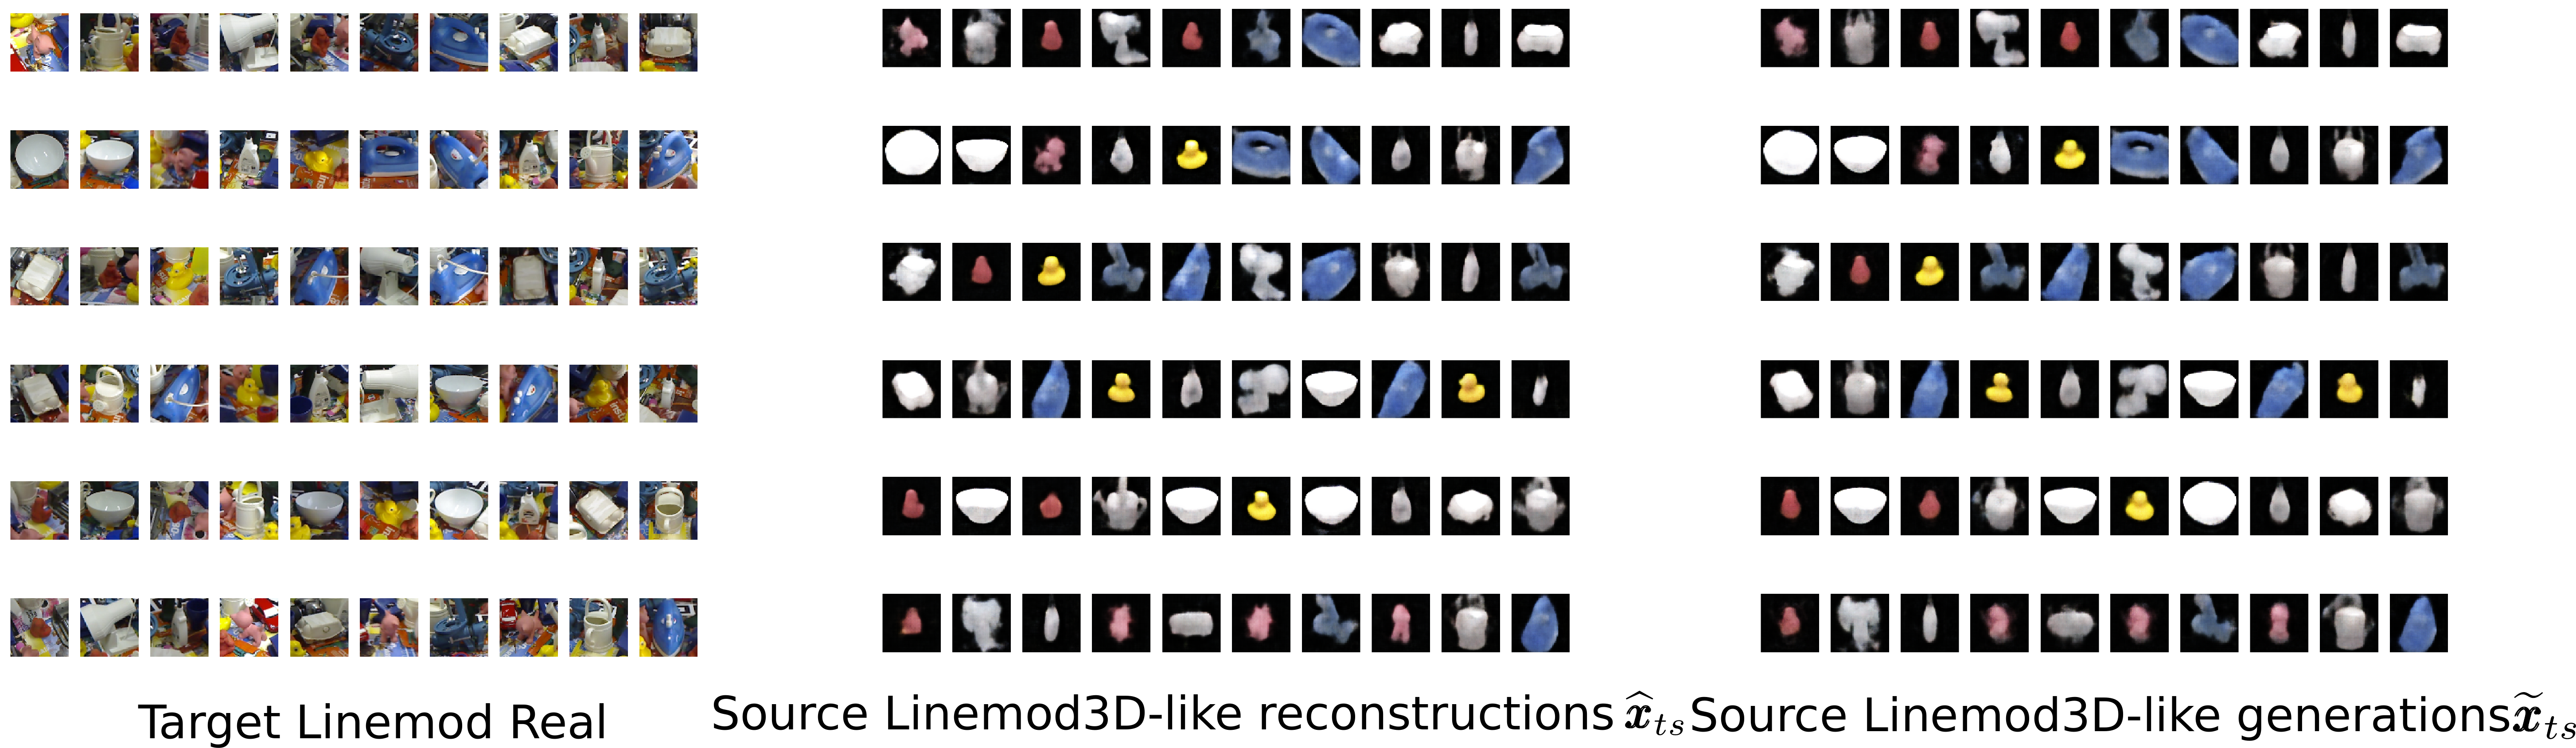}
   \caption{More Generations in task Linemod3D(source) -- LinemodReal(target)}
   \label{fig:linemod_more}
\end{figure*}

\begin{figure*}[thbp]
   \centering
   \includegraphics[width=1.0\textwidth]{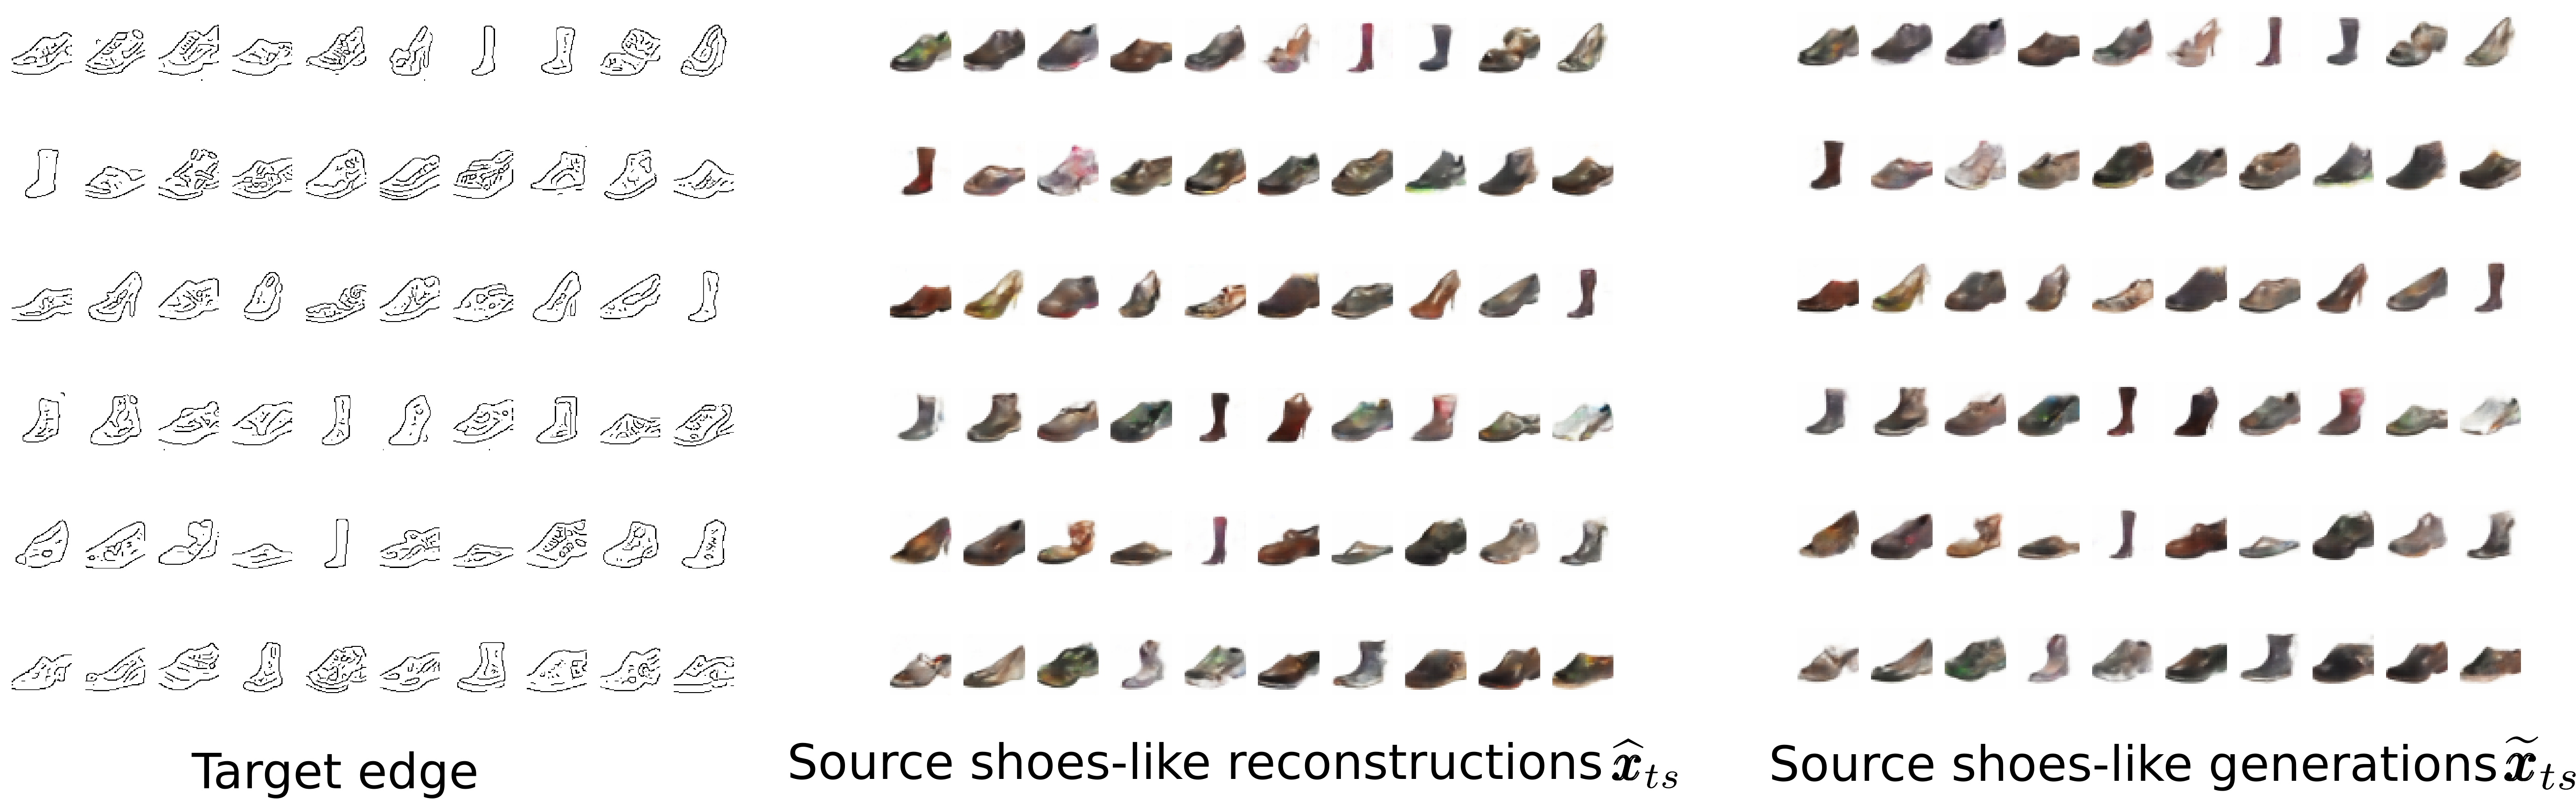}
   \caption{More Generations in task Shoes(source) -- edge(target)}
   \label{fig:shoes_edge_more}
\end{figure*}

\begin{figure*}[thbp]
   \centering
   \includegraphics[width=1.0\textwidth]{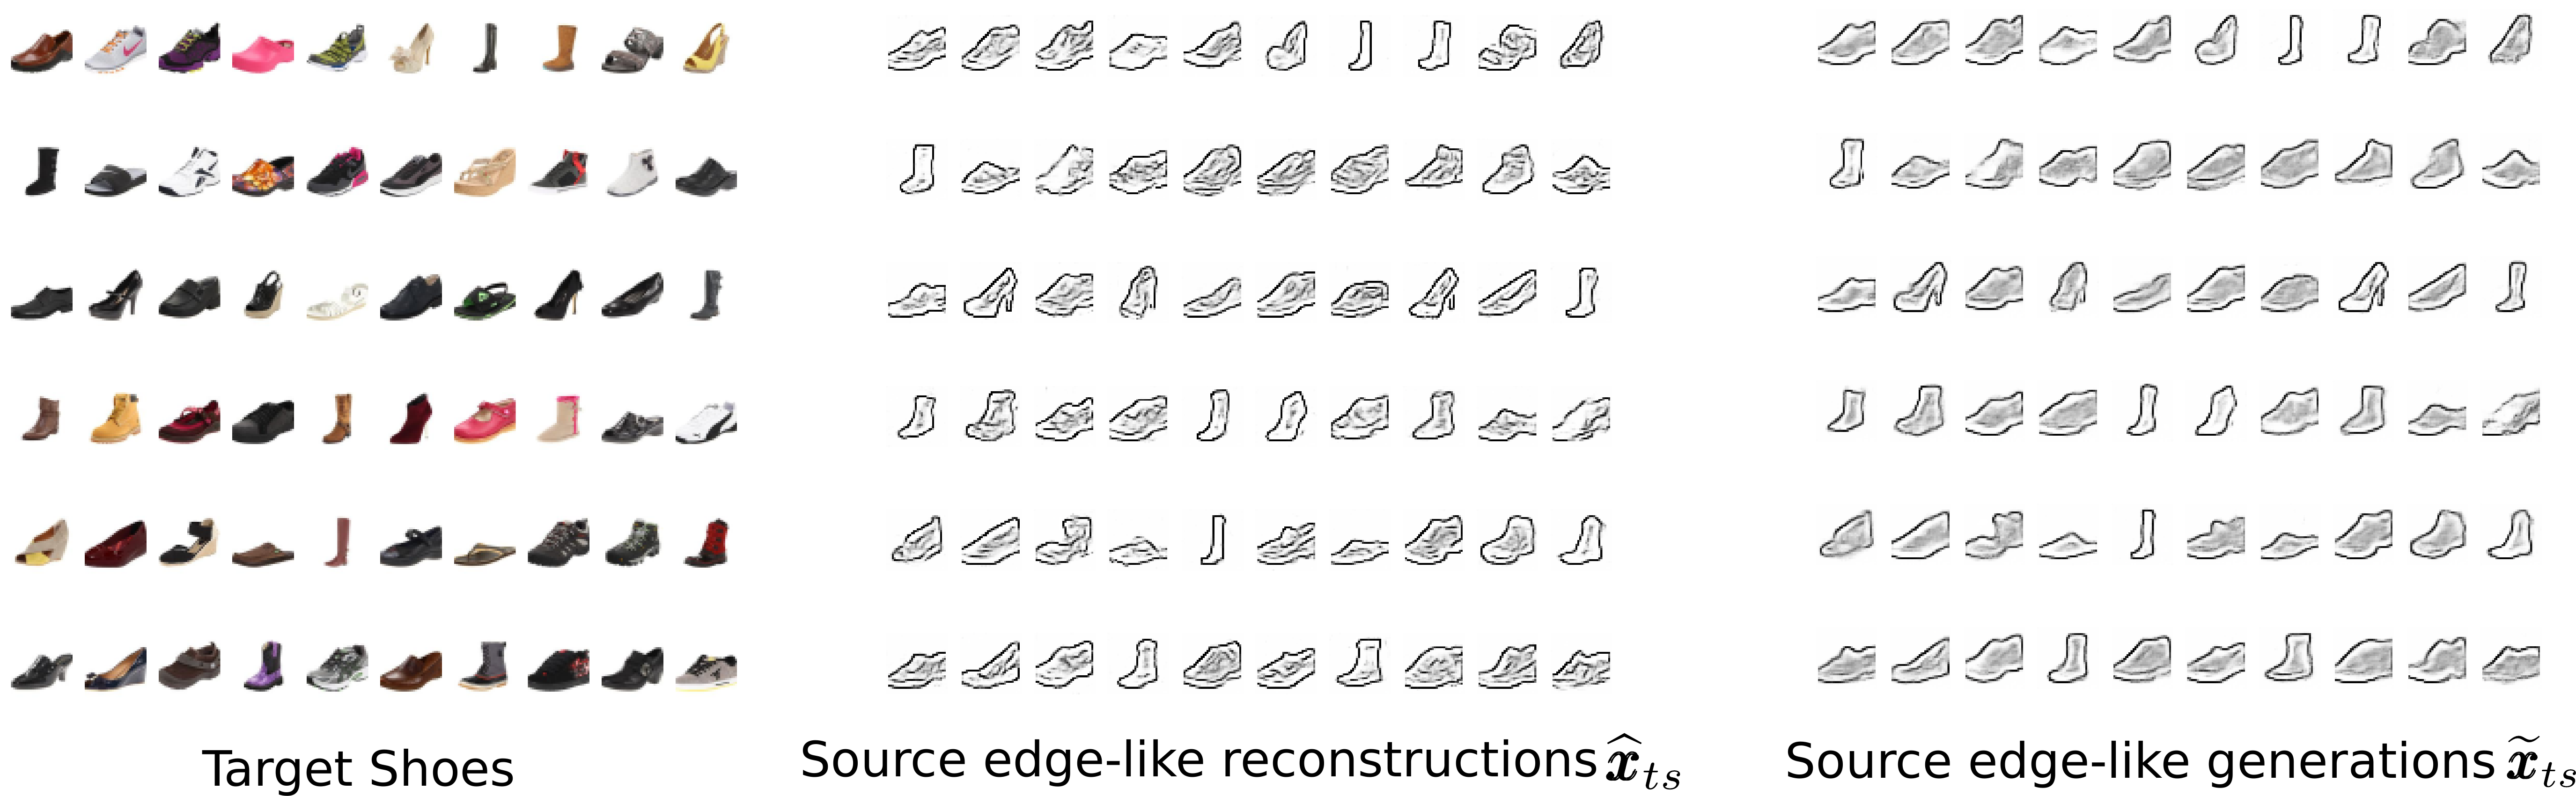}
   \caption{More Generations in task edge(source) -- Shoes(target)}
   \label{fig:edge_shoes_more}
\end{figure*}

\begin{figure*}[thbp]
   \centering
   \includegraphics[width=1.0\textwidth]{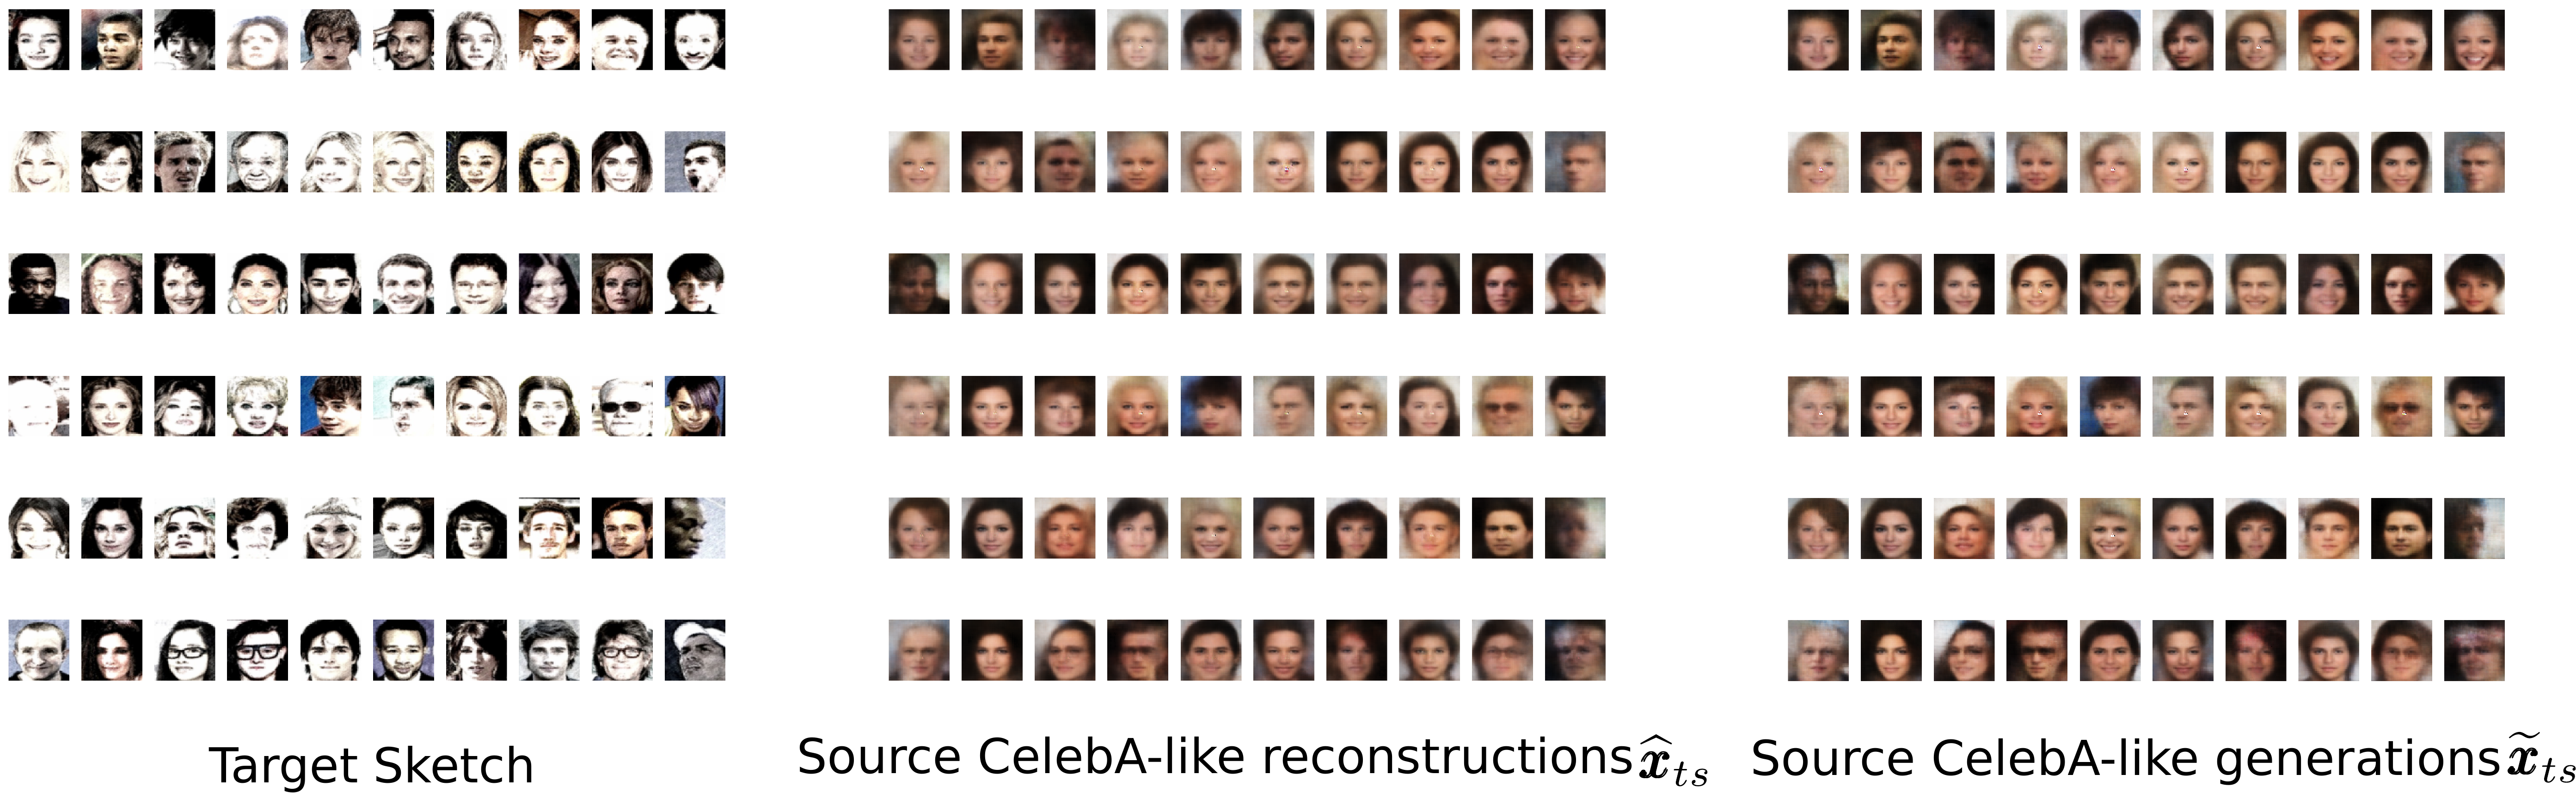}
   \caption{More Generations in task CelebA(source) -- Sketch(target)}
   \label{fig:face_sketch_more}
\end{figure*}

\begin{figure*}[thbp]
   \centering
   \includegraphics[width=1.0\textwidth]{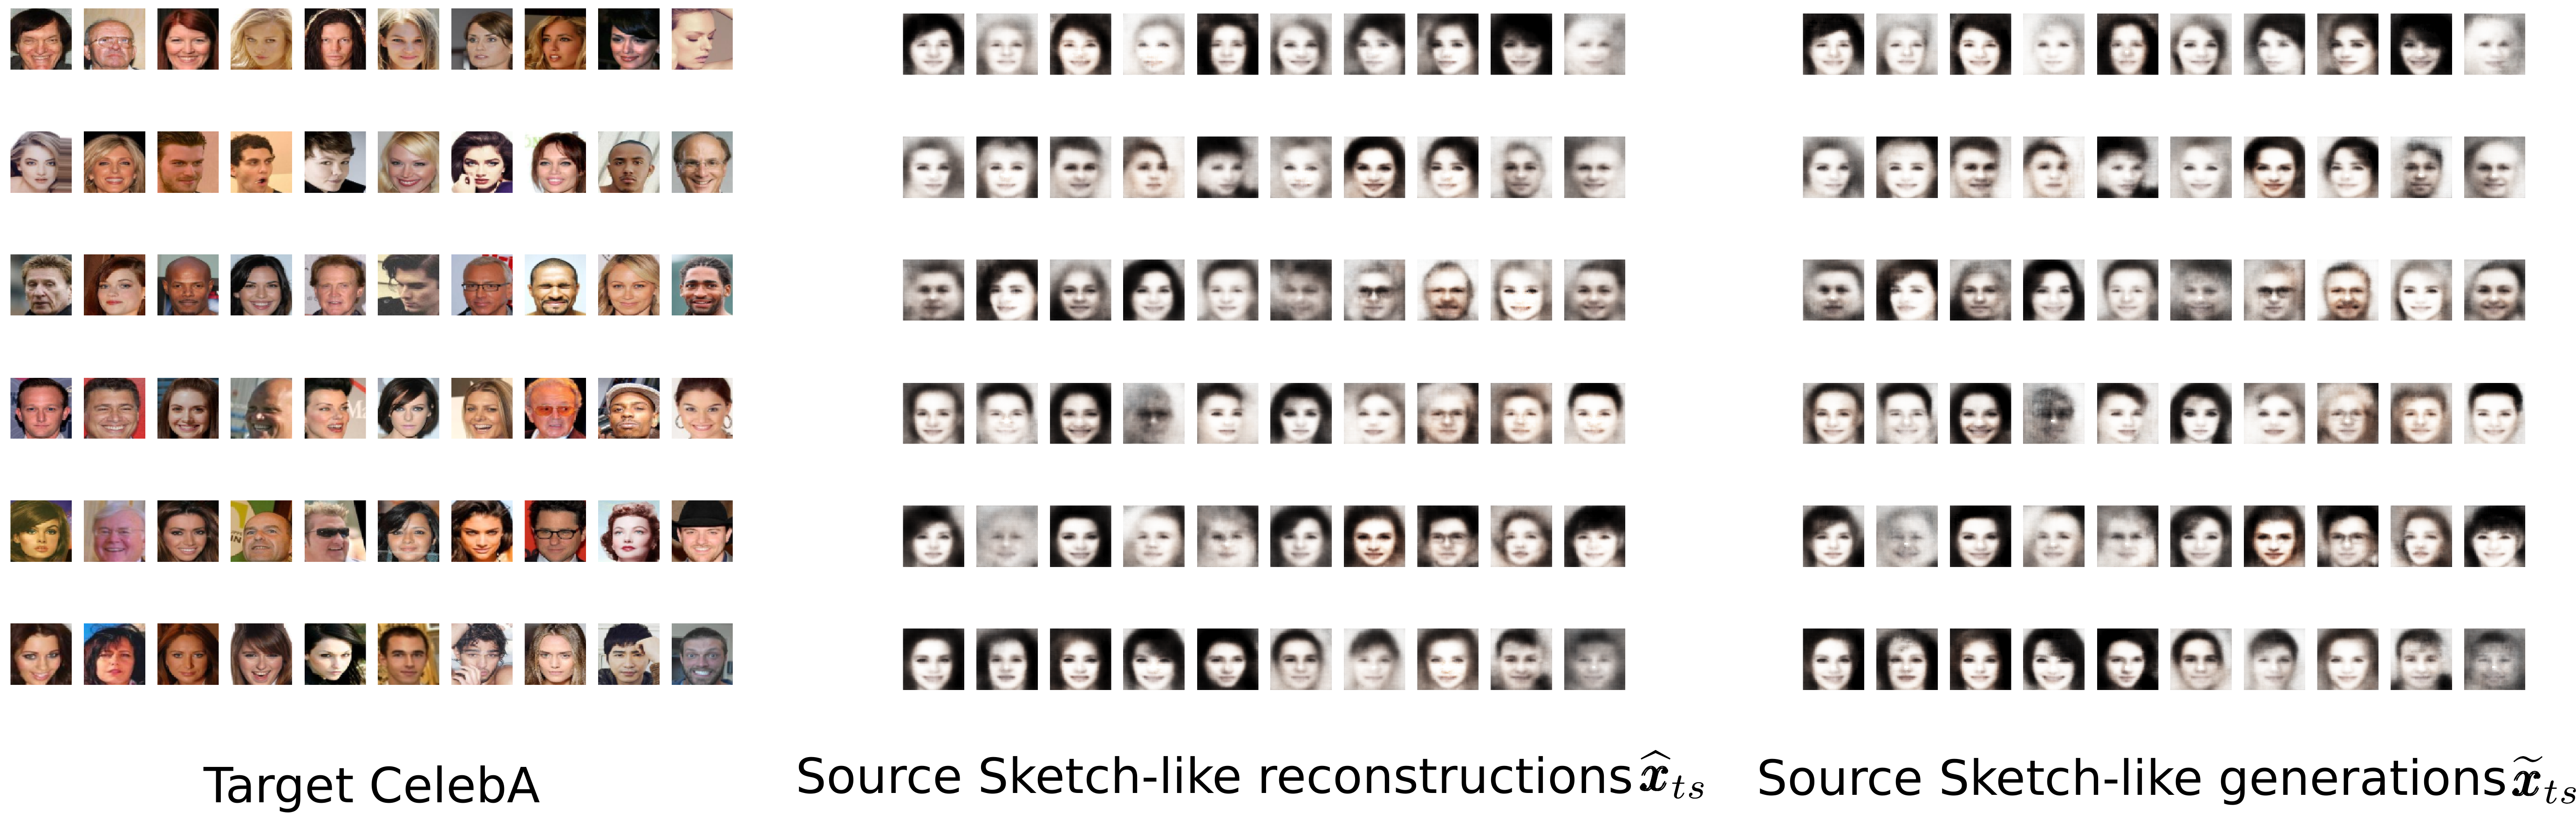}
   \caption{More Generations in task Sketch(source) -- CelebA(target)}
   \label{fig:sketch_face_more}
\end{figure*}
